# Supplementary material for: Practical application improvement to Quantum SVM: theory to practice
Source: arXiv:2012.07725 source file (2020-12-14)
Supplement: Supplementary file 1 [file supplementary.tex]

% \mtcsettitle{secttoc}{Supplementary Material Contents}
% \dosecttoc
% \secttoc
\section{Supplementary Material}
% \secttoc
% \setcounter{tocdepth}{4}
% \appendix the document TOC
% \part{Appendix} % Start the appendix part
% \tableofcontents
% \addcontentsline{toc}{chapter}{Network Architectures and Learning}
The following sections are included in this supplementary materials document:
\begin{itemize}
    \item \textbf{Section \ref{sub:dataset details} - Dataset details}: More detailed  description of the data sets used and their setups, including table listing the attributes of the data.
    \item \textbf{Section \ref{subsec:evaluation metrics} -  Evaluation metrics}: Complete details and formulas for the different evaluation metrics used in the experiments.
\end{itemize}

% The bibliography is reproduced at the end for convenience, since the supplement is separate from the main paper.

\subsection{Dataset details}
\label{sub:dataset details}

Table \ref{table:dataset statistics} describes statistics of datasets used in our experiments. 

\begin{table}[ht!]
\begin{center}
\caption{Dataset statistics }
\label{table:dataset statistics}
\scriptsize
\begin{tabular}{  l | l  l  l  l  l  l}
Dataset & time steps $T$ & dimension $n$ & $\tau$ (number predicted steps) & k (rolling windows) & frequency & domain \\
\hline
Traffic & $10392$ & $963$ & $24$ & $7$ & hourly & $\RR^+$ \\
Electricity (large) & $25920$ & $370$ & $24$ & $7$ & hourly & $\RR^+$ \\
Electricity (small) & $5833$ & $370$ & $24$ & $7$ & hourly & $\RR^+$ \\
Solar & $7009$ & $137$ & $24$ & $7$ & hourly & $\RR^+$  \\
Taxi & $1488$ & $1214$ & $24$ &  $56$ & $30$-minutes & $\NN$  \\
Wiki (large) & $635$ & $115084$ & $14$ & $4$ & daily & $\NN$ \\
Wiki (small) & $792$ & $2000$ & $30$ & $5$ & daily & $\NN$ \\
\end{tabular}
\end{center}
\end{table}

\subsection{Evaluation metrics}
\label{subsec:evaluation metrics}
Here we describe the evaluation metrics used in more detail.

% \bibliographystyle{IEEEtran}
% {\small
% \bibliography{reference}}
